# Supplementary material for: Small-Footprint Open-Vocabulary Keyword Spotting with Quantized LSTM Networks
Source: arXiv:2002.10851 source file (2020-02-25)
Supplement: Supplementary file 1 [file appendices.tex]

% Can be used to pull up biographies so that the bottom of the last one
% is flush with the other column.
%\enlargethispage{-5in}

% if have a single appendix:
%\appendix[Proof of the Zonklar Equations]
% or
%\appendix  % for no appendix heading
% do not use \section anymore after \appendix, only \section*
% is possibly needed

% use appendices with more than one appendix
% then use \section to start each appendix
% you must declare a \section before using any
% \subsection or using \label (\appendices by itself
% starts a section numbered zero.)
%
\newpage
\appendices
\section{An experiment on the memory of the CTC-trained LSTMs}
\label{app:lstm-memory}
Appendix one text goes here.

% you can choose not to have a title for an appendix
% if you want by leaving the argument blank
\section{}
\label{app:embedding-perspective}
Appendix two text goes here.

\section{}
Appendix two text goes here.
